# Supplementary material for: Grounded Text-to-Image Synthesis with Attention Refocusing
Source: arXiv:2306.05427 source file (2023-12-02)
Supplement: Supplementary file 1 [file 7_appendix.tex]

\begin{table*}
\centering
    \caption{Quantitative results in HRS benchmark spatial, size, color compositions}
    \label{tab:spatial_hrs}
    \begin{tabular}{lcccccccccccccc}
    \toprule
    \multirow{2}{*}{Model} & \multirow{2}{*}{CAR\linebreak \&SAR } & \multicolumn{4}{c}{\textbf{Spatial}} & \multicolumn{4}{c}{\textbf{Size}} & \multicolumn{4}{c}{\textbf{Color}} \\
     \cmidrule(r){3-6} \cmidrule(r){7-10} \cmidrule(r){11-14} 
     & & Easy & Medium& Hard& Average & Easy & Medium& Hard& Average& Easy  & Medium& Hard & Average  \\
    \midrule
    \multirow{2}{*}{Stable Diffusion} &   &20.96   & 4.19  & 0.29  & 8.48  &  26.95 & 0.60 & 0.00 & 9.18 & 18.37 & 11.78 & 7.68 & 12.61 \\
    
    &\checkmark& 47.90 &20.66&4.79&24.45 &43.11&6.59 &1.19 &16.97 &   35.24 & 20.16 &15.21& 23.54\\
    \midrule
    \multirow{2}{*}{Attend-and-excite} & & 23.65   & 5.09  & 1.20  & 9.98  & 26.946 & 2.9940  & 1.80 &10.58& 30.12 & 16.97 & 11.60 & 19.56\\
    &\checkmark& 43.41 & 15.57 & 3.29 & 20.76 &37.13 & 4.79 &0.60 &14.17 & 32.22 & 18.36 & 11.89 & 20.83\\
    \midrule
    \multirow{2}{*}{Layout-guidance }&  & 40.42&8.98&0.00 & 16.47 & 31.14 & 5.39 & 0.60 & 12.38 &24.70 & 10.78 & 7.68 & 14.39\\
    &\checkmark& 55.38 & 20.05 & 2.0958 &25.84&40.1&5.39 &1.19 & 15.56 &37.04 & 16.17 & 11.30 & 21.50 \\
    \midrule
    \multirow{2}{*}{Multi-diffusion} & & 35.63 & 6.89 & 0.90 & 14.47& 31.13 & 0.60 & 0.00 & 10.58 & 25.30 & 17.56 &8.58 & 17.15\\
    &\checkmark &50.29 & 16.76 &  0.898  & 22.6546 & 29.94 &2.40 & 0.00 &10.78 & 40.66 & 20.75 & 12.34 &24.59\\
    \midrule
    \multirow{2}{*}{GLIGEN} & & 66.47 & 45.21 & 25.45 & 45.71& 64.07 & 28.74 & 15.57& 36.13 & 24.40 & 17.37 & 11.74 & 17.84\\
    & \checkmark&72.15& 55.38 & 35.03 & 54.19 & 62.27 & 34.73& 22.155  & 39.72 & 42.16 & 28.74 & 17.47 & 29.46  \\
    % GLIGEN  & \checkmark & & & 81.40& 84.85 & 82.86 & 78.81& 58.04& 43.93 & 80.08 & 68.932 &  57.42 &  83.04 & 60.26 & 68.81\\
    % GLIGEN &\checkmark &\checkmark& &82.75 & 86.17 & 85.75 & 79.61 & 59.60 & 47.60 & 81.15& 70.47 & 61.22 &  84.89 & 62.27 & 70.94\\

    % \midrule
    % Deep-floy\\
    % Deep-floy loss\\

    \bottomrule
    \end{tabular}
\end{table*}
